# Supplementary material for: SoftCLIP: Softer Cross-modal Alignment Makes CLIP Stronger
Source: arXiv:2303.17561 source file (2023-12-16)
Supplement: Supplementary file 1 [file appendixcam.tex]

%\begin{figure*}[t]
%    \centering
%    \includegraphics[width = 0.95\textwidth]{iccv2023AuthorKit/figures/word_cam.pdf}
%    \caption{.}
%    \label{cam}
%\end{figure*}

\begin{figure}[t]
    \centering
    \includegraphics[width=8.2cm]{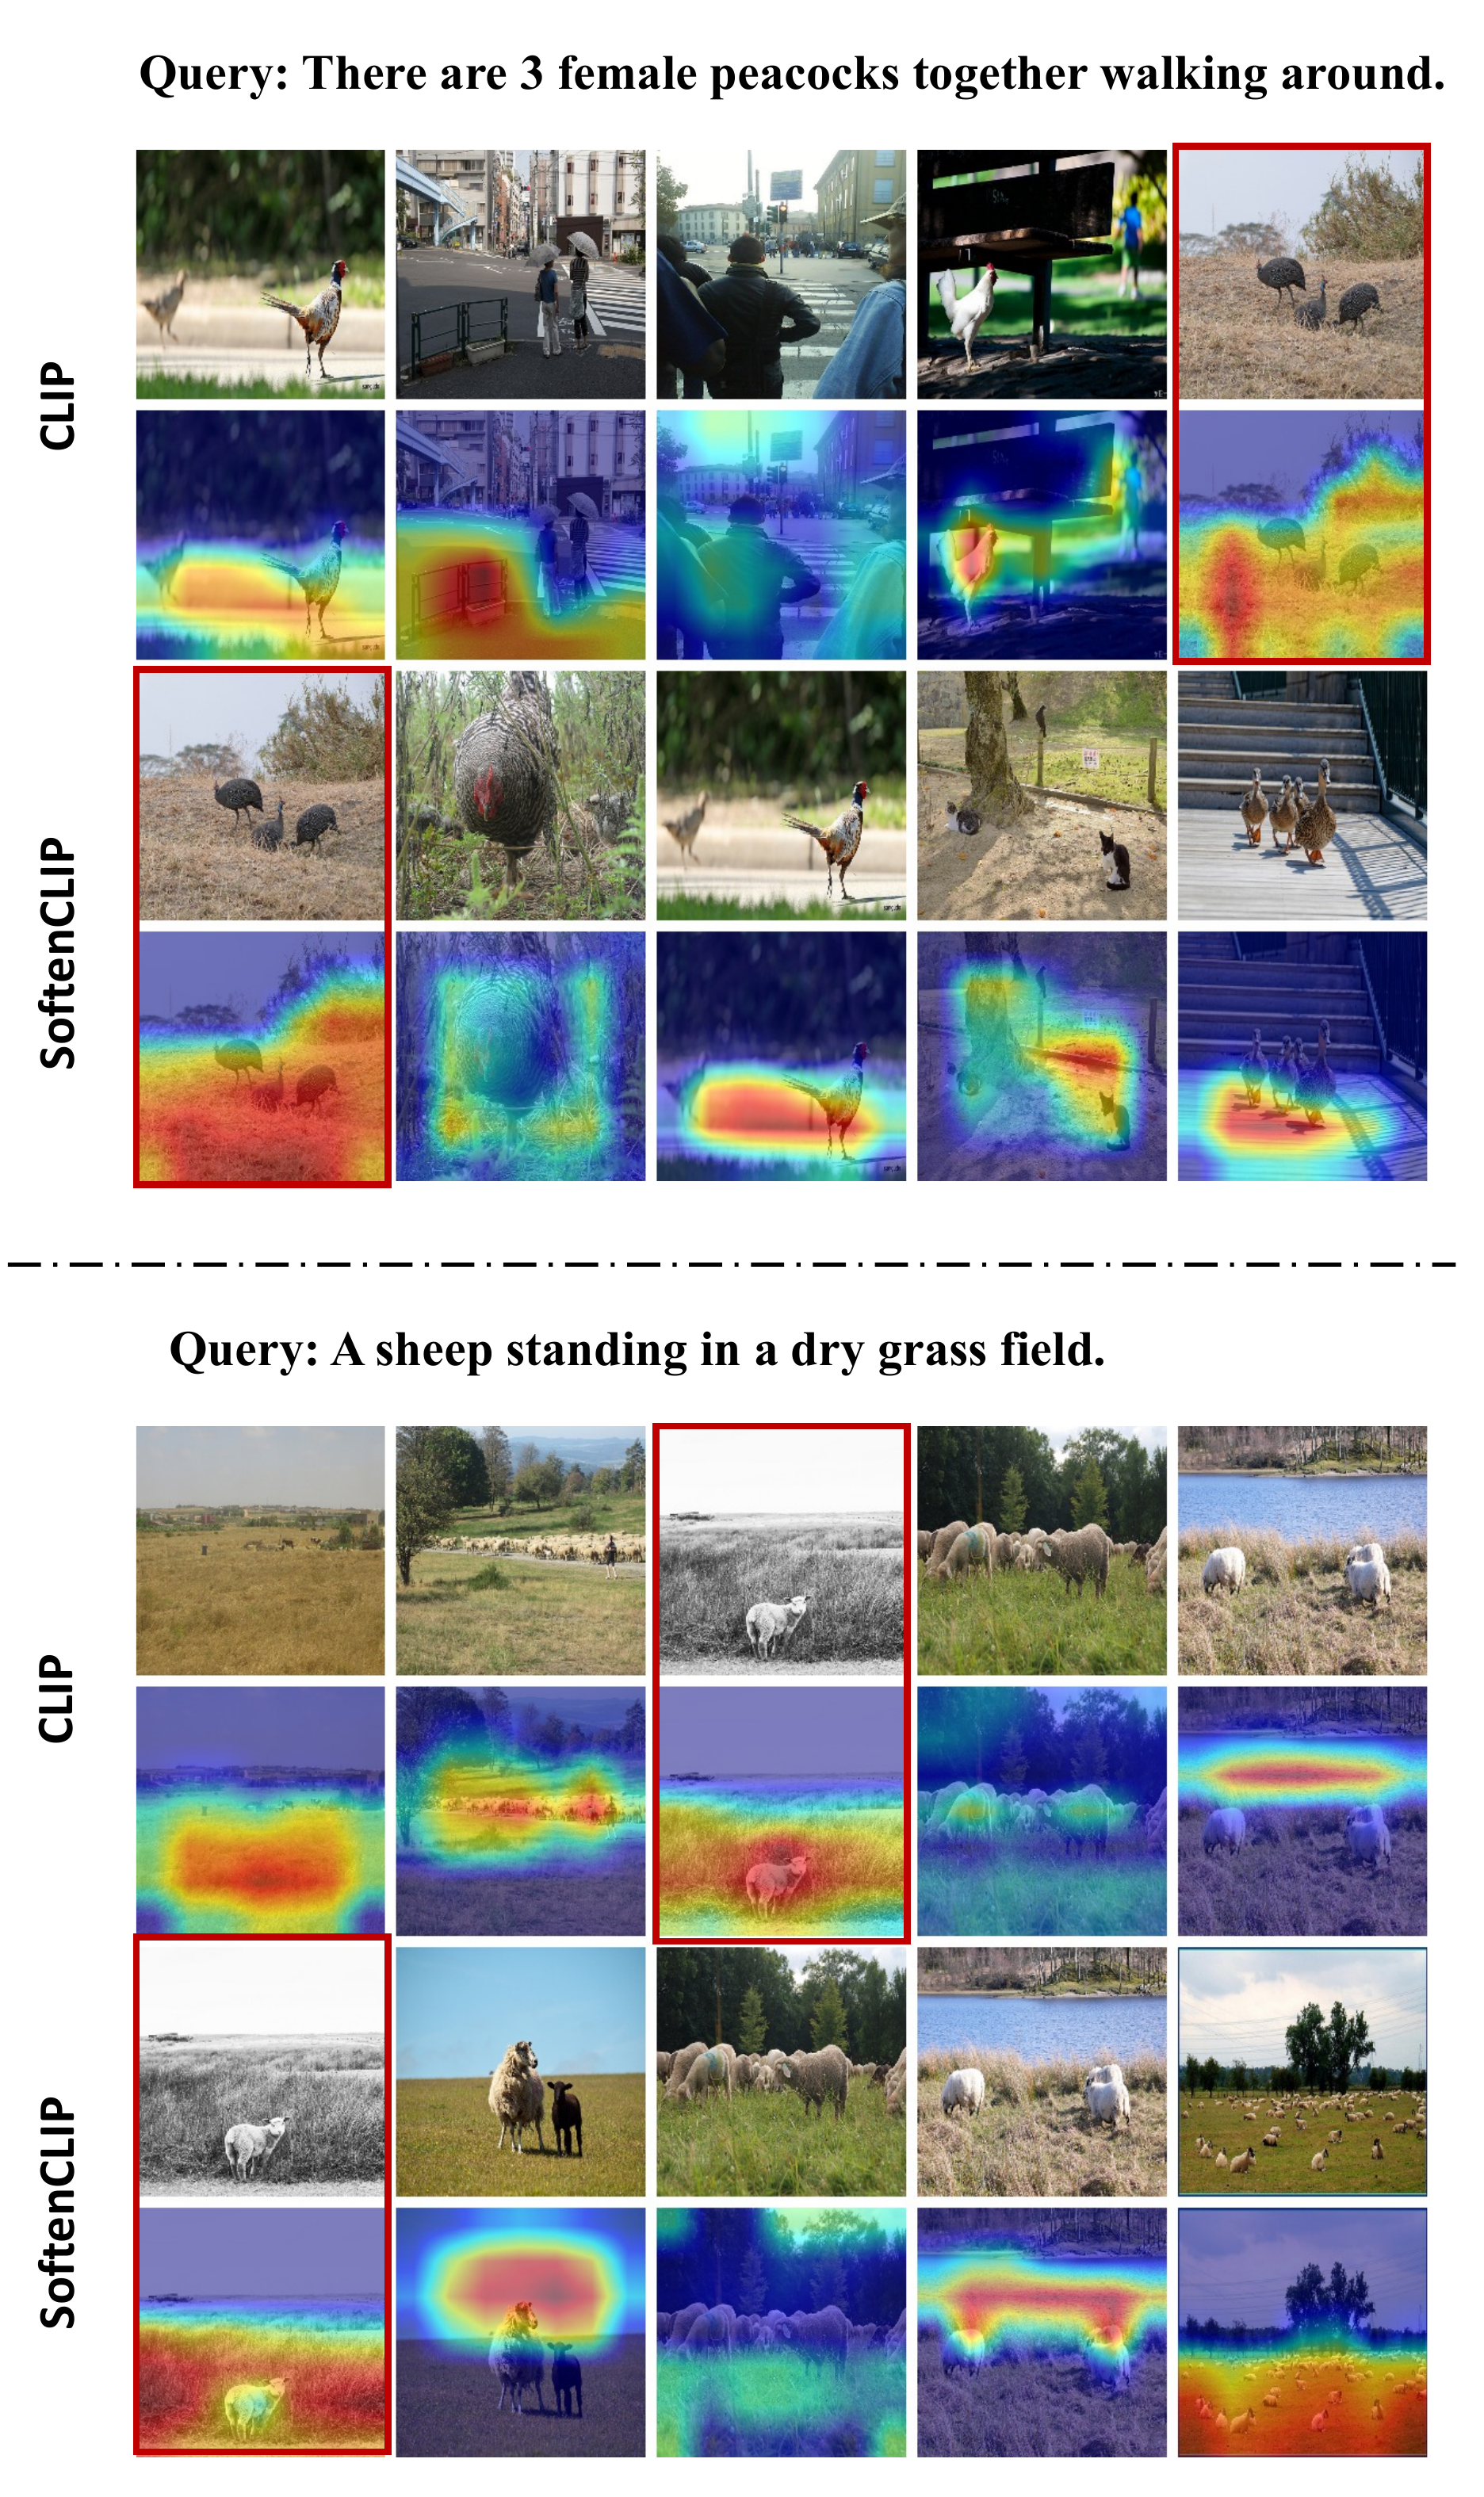}
    \caption{Grad-CAM visualizations.}
    \label{cam}
\end{figure}
